# Supplementary material for: A Path Integral approach to Quantum Fluid Dynamics
Source: arXiv:2002.00255 source file (2021-02-13)
Supplement: Supplementary file 1 [file appendix.tex]

\begin{widetext}

\section*{Appendix A: Computation for Second Order}

In this appendix we elaborate on how to expand the $j$ sum in equation (14) using multinomial theorem.

\begin{multline}
        \sum_{k=1}^{\infty}\frac{1}{k!}
        \Big(\frac{-i\epsilon}{\hbar}\Big)^k \lim_{n \rightarrow\infty} \Big(\prod_{j=1}^n\frac{1}{A_j}\Big) \int^{\infty}_{-\infty}\cdots\int^{\infty}_{-\infty} \exp\big( \frac{i\epsilon}{\hbar}\sum_{j=1}^n \Big[\frac{M}{2\epsilon^2} (y_j-y_{j-1})^2  -\frac{y_j^2}{2!} \frac{\partial^2}{\partial x^2}V(x)|_{x=x^{cl}_j}\Big]\big)
        \\ \times \Big[ \sum_{\sum P_m=k}\frac{k!}{P_3!P_4!\cdots}\prod_{m=3}^{\infty} \Big(\sum_{j=1}^n\frac{1}{m!} \frac{\partial^m}{\partial x^m}V(x)|_{x=x^{cl}_j} \;\;y_j^{m}\Big)^{P_m} \Big] dy_1\cdots dy_n
\end{multline}

The primary aim is to express each order of $k$, as sum of integrals of the form (18). The object we need to expand by multinomial theorem is,

\begin{align}
    \sum_{\sum P_m=k}\frac{k!}{P_3!P_4!\cdots}\prod_{m=3}^{\infty} \Big(\sum_{j=1}^n\frac{1}{m!} \frac{\partial^m}{\partial x^m}V(x)|_{x=x^{cl}_j} y_j^{m}\Big)^{P_m}
\end{align}
    Now each sum of the form $\Big(\sum_{j=1}^n\frac{1}{m!} \frac{\partial^m}{\partial x^m}V(x)|_{x=x^{cl}_j} y_j^{m}\Big)^{P_m}$ can be brocken down by multinomial theorem as,
    
\begin{align*}
    &\prod_{m=3}^\infty \Big(\sum_{j=1}^n\frac{1}{m!} \frac{\partial^m}{\partial x^m}V(x)|_{x=x^{cl}_j} y_j^{m}\Big)^{P_m}\\
    =&\prod_{m=3}^\infty \frac{1}{m!^{P_m}}\Big(\sum_{j=1}^n \frac{\partial^m}{\partial x^m}V(x)|_{x=x^{cl}_j} y_j^{m}\Big)^{P_m}\\
    =&\prod_{m=3}^\infty \frac{1}{m!^{P_m}}\Big(\sum_{\sum l^j_m= P_m}\frac{P_m!}{l^1_m!l^2_m!\cdots l^n_m!}    \prod_{j=1}^n \Big(\frac{\partial^m}{\partial x^m}V(x)|_{x=x^{cl}_j} y_j^{m}\Big)^{l^j_m}\Big)
\end{align*}

So Equation (47) can be rewritten as,

\begin{align}
    \sum_{\sum P_m=k}\frac{k!}{P_3!P_4!\cdots} \prod_{m=3}^\infty \frac{1}{m!^{P_m}}\Big(\sum_{\sum l^j_m= P_m}\frac{P_m!}{l^1_m!l^2_m!\cdots l^n_m!}    \prod_{j=1}^n \Big(\frac{\partial^m}{\partial x^m}V(x)|_{x=x^{cl}_j} y_j^{m}\Big)^{l^j_m}\Big)
\end{align}

This is essentially an expansion of the second line of equation (46). Now assume $k=2, j=1,2$ and $m=3,4$. Then equation (48) becomes,

\begin{align*}
    &\sum_{\sum P_m=2}\frac{2!}{P_3!P_4!} \Big(\frac{1}{3!^{P_3}4!^{P_4}}\Big)\prod_{m=3}^4 \Big(\sum_{\sum l^j_m= P_m}\frac{P_m!}{l^1_m!l^2_m!} \prod_{j=1}^2 \Big(\frac{\partial^m}{\partial x^m}V(x)|_{x=x^{cl}_j} y_j^{m}\Big)^{l^j_m}\Big)\\
    =&\frac{2!}{2!}\Big(\frac{1}{3!^{2}}\Big)\Big(\sum_{\sum l^j_3= 2}\frac{2!}{l^1_3!l^2_3!} \prod_{j=1}^2 \Big(\frac{\partial^3}{\partial x^3}V(x)|_{x=x^{cl}_j} y_j^{3}\Big)^{l^j_3}\Big)\\
    +&\frac{2!}{1!1!}\Big(\frac{1}{3!4!}\Big)\Big(\sum_{\sum l^j_3= 1}\frac{1!}{l^1_3!l^2_3!} \prod_{j=1}^2 \Big(\frac{\partial^3}{\partial x^3}V(x)|_{x=x^{cl}_j} y_j^{3}\Big)^{l^j_3}\Big)\Big(\sum_{\sum l^j_4= 1}\frac{1!}{l^1_4!l^2_4!} \prod_{j=1}^2 \Big(\frac{\partial^4}{\partial x^4}V(x)|_{x=x^{cl}_j} y_j^{4}\Big)^{l^j_4}\Big)\\
    +&\frac{2!}{2!}\Big(\frac{1}{4!^2}\Big)\Big(\sum_{\sum l^j_4= 2}\frac{2!}{l^1_4!l^2_4!} \prod_{j=1}^2 \Big(\frac{\partial^4}{\partial x^4}V(x)|_{x=x^{cl}_j} y_j^{4}\Big)^{l^j_4}\Big)
\end{align*}
\begin{align*}
    =&\frac{2!}{2!}\Big(\frac{1}{3!^{2}}\Big)
    \Bigg(\frac{2!}{2!} \Big(\frac{\partial^3}{\partial x^3}V(x)|_{x=x^{cl}_1} y_1^{3}\Big)^{2}
    +\frac{2!}{1!1!}   \Big(\frac{\partial^3}{\partial x^3}V(x)|_{x=x^{cl}_1} y_1^{3}\Big)\Big(\frac{\partial^3}{\partial x^3}V(x)|_{x=x^{cl}_2} y_2^{3}\Big)
    +\frac{2!}{2!}     \Big(\frac{\partial^3}{\partial x^3}V(x)|_{x=x^{cl}_2} y_2^{3}\Big)^{2}
    \Bigg)\\
    +&\frac{2!}{1!1!}\Big(\frac{1}{3!4!}\Big)\Bigg(\Big(\frac{\partial^3}{\partial x^3}V(x)|_{x=x^{cl}_1} y_1^{3}+\frac{\partial^3}{\partial x^3}V(x)|_{x=x^{cl}_2} y_2^{3}\Big)\Big(\frac{\partial^4}{\partial x^4}V(x)|_{x=x^{cl}_1} y_1^{4}+\frac{\partial^4}{\partial x^4}V(x)|_{x=x^{cl}_2} y_2^{4}\Big)\Bigg)\\
    +&\frac{2!}{2!}\Big(\frac{1}{4! ^2}\Big)\Bigg(\frac{2!}{2!} \Big(\frac{\partial^4}{\partial x^4}V(x)|_{x=x^{cl}_1} y_1^{4}\Big)^{2}
    +\frac{2!}{1!1!}   \Big(\frac{\partial^4}{\partial x^4}V(x)|_{x=x^{cl}_1} y_1^{4}\Big)\Big(\frac{\partial^4}{\partial x^4}V(x)|_{x=x^{cl}_2} y_2^{4}\Big)
    +\frac{2!}{2!}     \Big(\frac{\partial^4}{\partial x^4}V(x)|_{x=x^{cl}_2} y_2^{4}\Big)^{2}
    \Bigg)\\
\end{align*}

\begin{align*}
    =& \Big(\frac{1}{3!}\Big)^{2}
    \Bigg( \Big(\frac{\partial^3}{\partial x^3}V(x)|_{x=x^{cl}_1} \Big)^{2} y_1^{6}
    +     2\Big(\frac{\partial^3}{\partial x^3}V(x)|_{x=x^{cl}_1} \frac{\partial^3}{\partial x^3}V(x)|_{x=x^{cl}_2} \Big) y_1^{3} y_2^{3}
    +      \Big(\frac{\partial^3}{\partial x^3}V(x)|_{x=x^{cl}_2} \Big)^{2} y_2^{6}
    \Bigg)\\
    +& \Big(\frac{2}{3!4!}\Big) 
    \Bigg( 
    \Big(\frac{\partial^3}{\partial x^3}V(x)|_{x=x^{cl}_1}\frac{\partial^4}{\partial x^4}V(x)|_{x=x^{cl}_1}\Big) \;\;y_1^{7}
    +\Big(\frac{\partial^3}{\partial x^3}V(x)|_{x=x^{cl}_2}\frac{\partial^4}{\partial x^4}V(x)|_{x=x^{cl}_2}\Big) \;\;y_2^{7}\\
    &+\Big(\frac{\partial^3}{\partial x^3}V(x)|_{x=x^{cl}_1}\frac{\partial^4}{\partial x^4}V(x)|_{x=x^{cl}_2}\Big) \;\;y_1^{3}y_2^{4}
    +\Big(\frac{\partial^4}{\partial x^4}V(x)|_{x=x^{cl}_1}\frac{\partial^3}{\partial x^3}V(x)|_{x=x^{cl}_2}\Big) \;\;y_1^{4}y_2^{3}
    \Bigg)\\
    +& \Big(\frac{1}{4!}\Big)^2
    \Bigg(  \Big(\frac{\partial^4}{\partial x^4}V(x)|_{x=x^{cl}_1} \Big)^{2}  y_1^{8}
    +      2\Big(\frac{\partial^4}{\partial x^4}V(x)|_{x=x^{cl}_1} \frac{\partial^4}{\partial x^4}V(x)|_{x=x^{cl}_2} \Big) y_1^{4} y_2^{4}
    +       \Big(\frac{\partial^4}{\partial x^4}V(x)|_{x=x^{cl}_2} \Big)^{2}  y_2^{8}
    \Bigg)
\end{align*}

This clearly shows the order 2 can be expressed as sum of the integrals of the form (18), all of which can be carried out in closed form. The generalisation to higher orders (denoted by k index), more moments (denoted by j index), or higher order non-vanishing derivatives (denoted by m index is straight forward) 
\end{widetext}
